# Supplementary material for: Sketch-Fill-A-R: A Persona-Grounded Chit-Chat Generation Framework
Source: arXiv:1910.13008 source file (2019-10-28)
Supplement: Supplementary file 1 [file 7-appendix.tex]

\section{Appendix}

\begin{figure*}[ht!]
    \begin{center}
        \includegraphics[width=\linewidth]{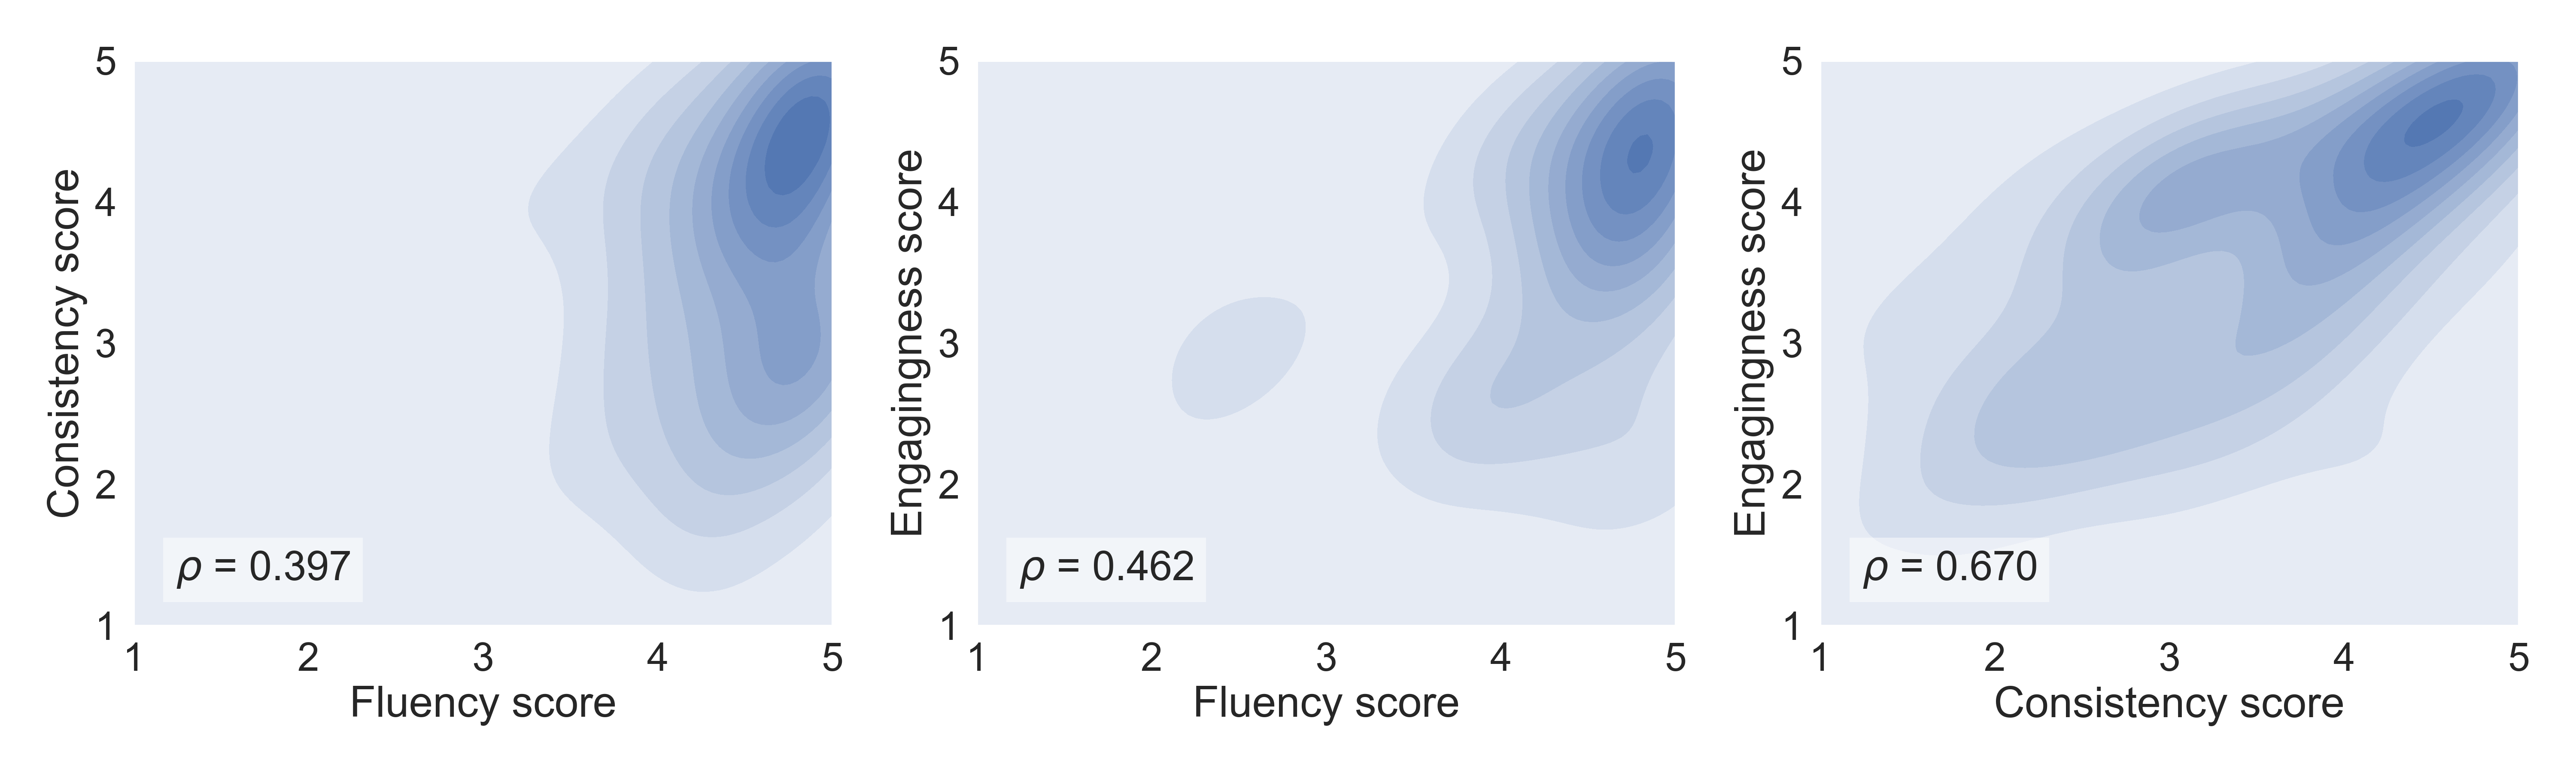}
    \end{center}
    \caption{ 
    % \COMM{Move 2 or all to appendix + add table with all correlation numbers.}
    % 
    Correlations between different dimensions in which model responses where rated. Plots include Pearson correlation coefficients ($\rho$) for each dimension pair. The data suggests weak to moderate correlation between \textit{fluency} and \textit{consistency}, and \textit{fluency} and \textit{engagingness} respectively, and strong correlation between \textit{engagingness} and \textit{consistency}.}
    \label{fig:corr-pairwise}
\end{figure*}

\begin{figure}[ht!]
    \begin{center}
        \includegraphics[width=\linewidth]{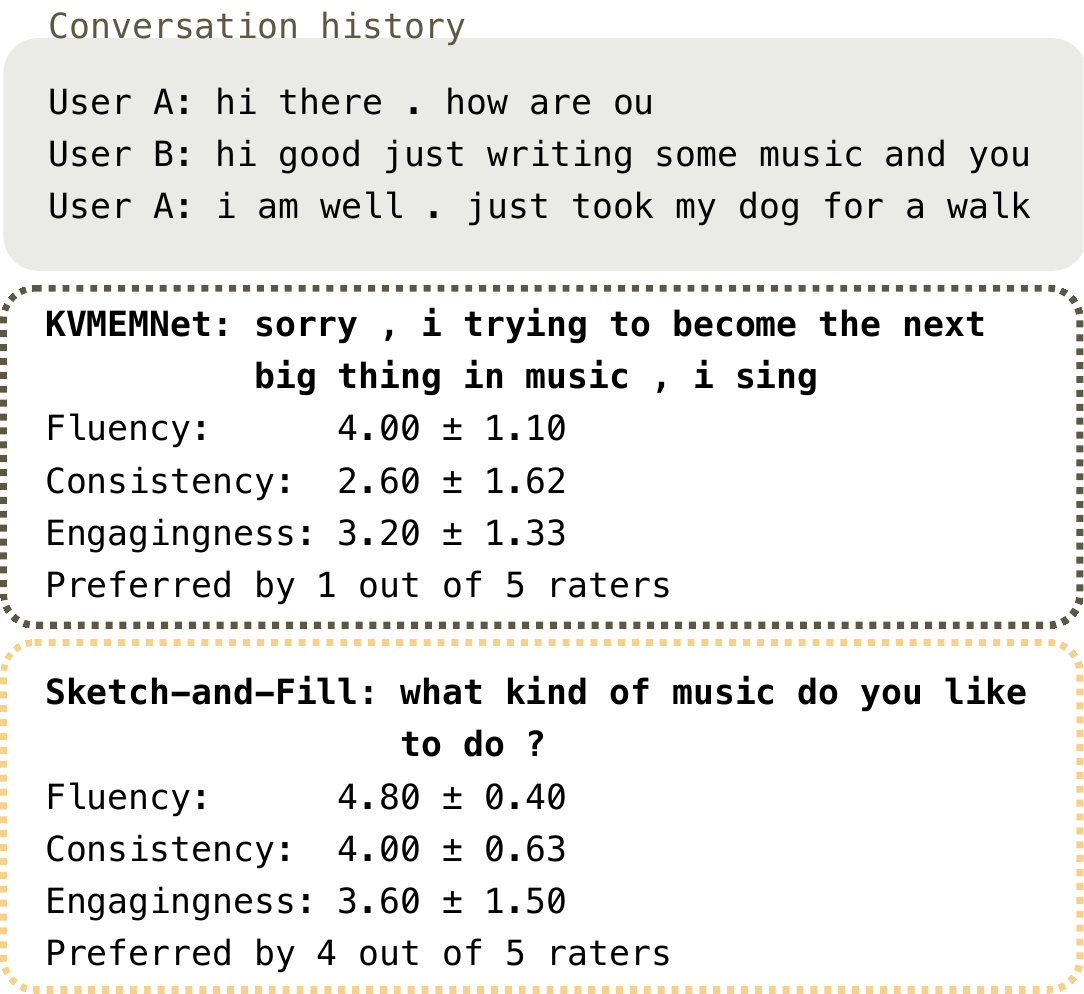}
    \end{center}
    \caption{Example conversations from the human user studies.}
    \label{fig:corr-pairwise}
\end{figure}

\subsection{Model Architecture and Training Parameters}
In all models we used single-layer LSTMs with hidden sizes of 300 throughout, and used GloVe embeddings of size 300. All Sketch-and-Fill models were trained with Adam initialized with learning rate 0.0001. We used batch sizes of 32. In single-turn experiments we used beam sizes of 7, and in multi-turn experiments we used beam sizes of 10. Dropout was applied for all models with probability 0.4. 

\subsection{Persona Preprocessing}
Persona traits were pre-processed to remove stop-words. These were initialized with the defaults from NLTK and augmented with top commonly seen words in persona traits. 

["and", "my", "i", "very", "is", "favorite", "to", "like", "go", "also", "i'm", "am", "a", "lot", "at", "the", "for", "when", "are", "this", "on", "just", ".", ",", "!", "?", "help", "play", "in", "have", "of", "by", "do", "one", "it", "an", "was", "me", "could", "be", "with", "but", "before", "after", "from", "i\'ve", "don\'t", "only", "love", "had", "i\'m", "over", "what", "as", "want", "into", "try", "whatever", "get", "t", "s", "no", "own", 'i', 'me', 'my', 'myself', 'we', 'our', 'ours', 'ourselves', 'you', 'your', 'yours', 'yourself', 'yourselves', 'he', 'him', 'his', 'himself', 'she', 'her', 'hers', 'herself', 'it', 'its', 'itself', 'they', 'them', 'their', 'theirs', 'themselves', 'what', 'which', 'who', 'whom', 'this', 'that', 'these', 'those', 'am', 'is', 'are', 'was', 'were', 'be', 'been', 'being', 'have', 'has', 'had', 'having', 'do', 'does', 'did', 'doing', 'a', 'an', 'the', 'and', 'but', 'if', 'or', 'because', 'as', 'until', 'while', 'of', 'at', 'by', 'for', 'with', 'about', 'against', 'between', 'into', 'through', 'during', 'before', 'after', 'above', 'below', 'to', 'from', 'up', 'down', 'in', 'out', 'on', 'off', 'over', 'under', 'again', 'further', 'then', 'once', 'here', 'there', 'when', 'where', 'why', 'how', 'all', 'any', 'both', 'each', 'few', 'more', 'most', 'other', 'some', 'such', 'no', 'nor', 'not', 'only', 'own', 'same', 'so', 'than', 'too', 'very', 's', 't', 'can', 'will', 'just', 'don', 'should', 'now']

\subsection{Number of Persona Tags}
Training: 124,298 words were converted to persona tags out of 1,505,395 words total. \\
Validation: 8,307 words were converted to persona tags out of 92,586 words total.

\subsection{Global-to-Local Memory Pointer Networks}
\cite{wu2018globaltolocal} construct a global memory distribution that acts as a mask over the memory and is concatenated with encoded dialogue history and memory information before initializing as the decoder's hidden state. They also construct a local memory pointer that identifies the word to retrieve. These auxiliary tasks are trained using cross-entropy loss. 

The global pointer label is defined $G^{label} = (g_{0}^{l},...,g_{i}^{l})$ as a vector where $g_{i}^{l}$ is 1 if the word is expected in $y_{t}^{*}$ and 0 otherwise.
Using the same notation as in Section 3.1, we compute the global pointer as follows:
\eq{
    & g_i = Sigmoid(((y_{t}, h_{t}^{d})^{T}e_{i}) \\
    & Loss_g = -\sum_{i=1}^{T}[g_{i}^{l} \times log(g_{i}) + (1 - g_{i}^{l}) \times log(1 - g_{i}] \\
}

This global pointer is used as a mask on the memory module before the decoding procedure $e_i = e_i \times g_i$. The local pointer label is used at every time step to identify which memory index (and thus word) to point to. If at $y^{*}_t$ a persona trait is expected, $L_{t}^{label}$ holds corresponding index, and is $m$ otherwise. 

\eq{
    & Loss_l = \sum_{t=1}^{m} -log(L_{t}(L_{t}^{label}) \label{eq:local_loss}
}

\subsection{Language Model Pretraining}
OpenAI GPT consists of a 12 layer Transformer and is pre-trained on the BooksCorpus dataset. 

\subsection{Ethical Implications}
During experiments, we identified a number of ethical implications for future work. 
The \texttt{Persona-Chat} dataset was noted by some raters to contain potentially inappropriate statements (e.g., "my wife spends all my money") and is based in US culture (e.g., food, music, cars, names).
It also lacked content to fail gracefully when it didn't have an appropriate response (e.g., "I'm sorry I don't understand," "I don't know"). 
As such, learned model responses were occasionally insensitive and confusing to human users.

\subsection{Visualizing Model Attention}
We visualize the three sets of attention weights in our model: the context weights in Figure \ref{fig:context_attention}, and memory weights and persona trait weights in Figure \ref{fig:memory_attention}. Figure \ref{fig:context_attention}'s x-axis shows a conversation ending with a question reflected by the user about hobbies. The response has high attention weights on \textit{hobbies} and the user's own \textit{garden} hobby in the previous context. Figure \ref{fig:memory_attention} (right) shows that in response to this \textit{hobbies} question, attention is first distributed over hobby-related personas before converging on the mountain biking persona trait over time. Finally, we observe in Figure \ref{fig:memory_attention} (left) that the memory attention is most heavily weighted on coffee, which may explain why the coffee persona begins with such high weights.

\begin{figure}
    \centering
    \includegraphics[width=\linewidth]{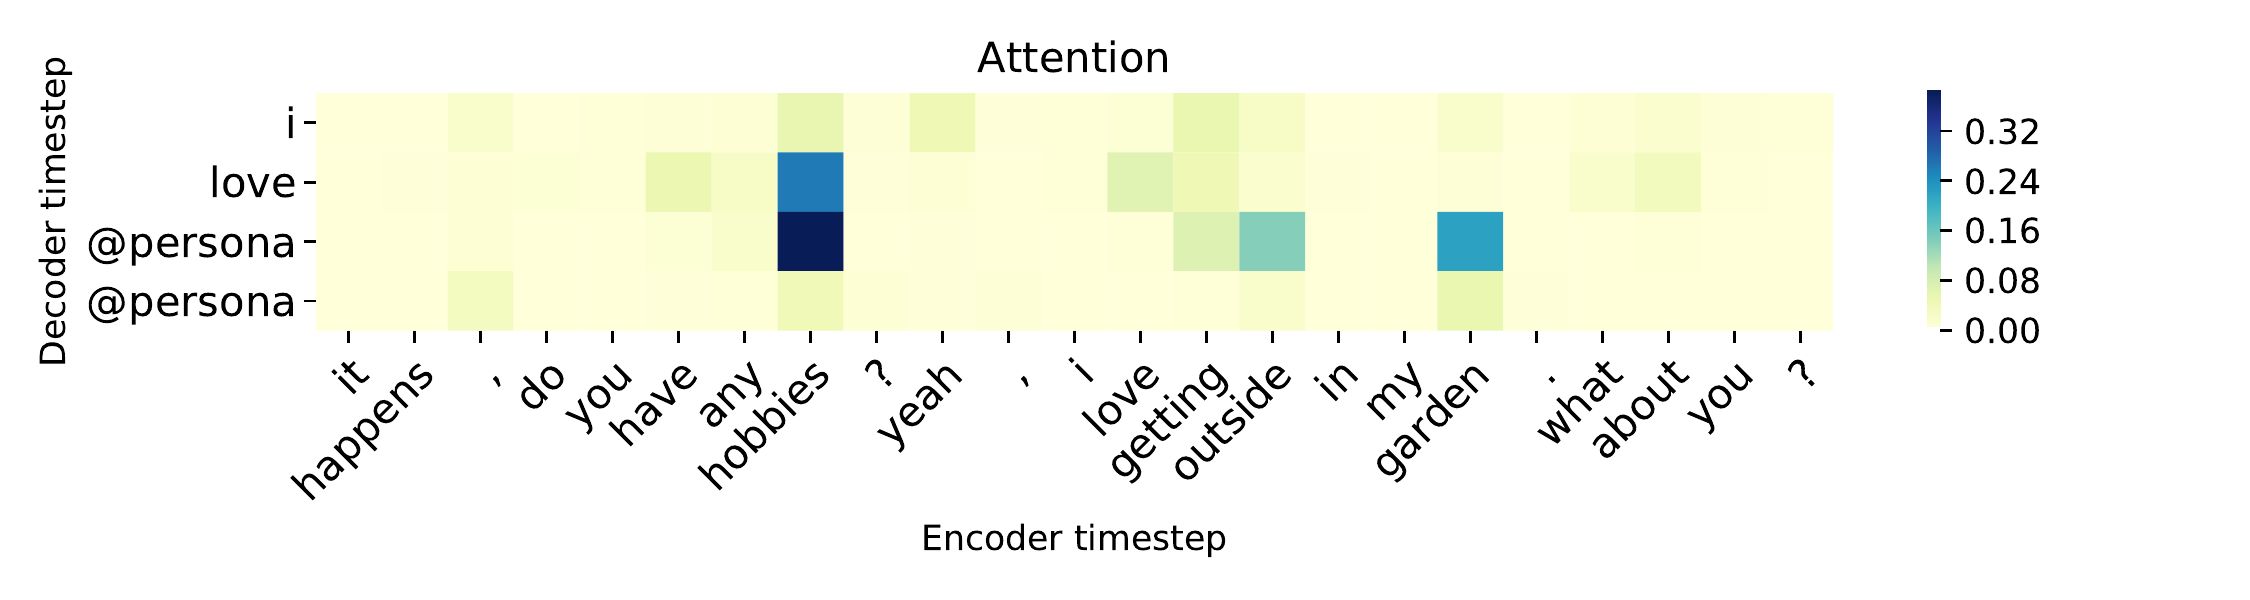}
    \caption{Attention weights over the previous context. Decoder timesteps are on the y-axis and encoder timesteps are on the x-axis. }
    \label{fig:context_attention}
\end{figure}
\begin{figure}
    \centering
    \begin{minipage}{0.4\linewidth}
        \includegraphics[height=100pt]{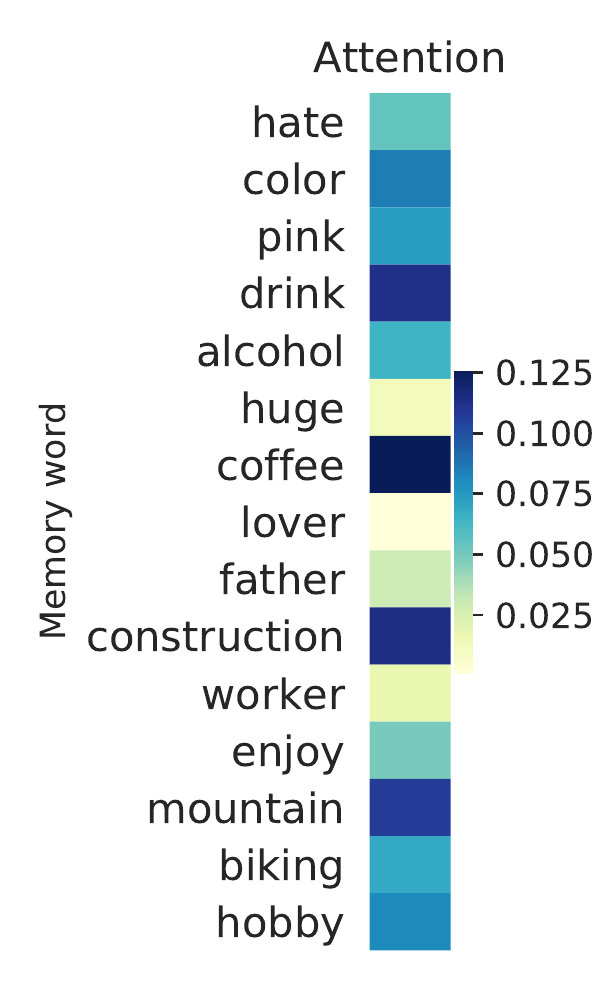}
    \end{minipage}
    \begin{minipage}{0.58\linewidth}
        \includegraphics[height=100pt]{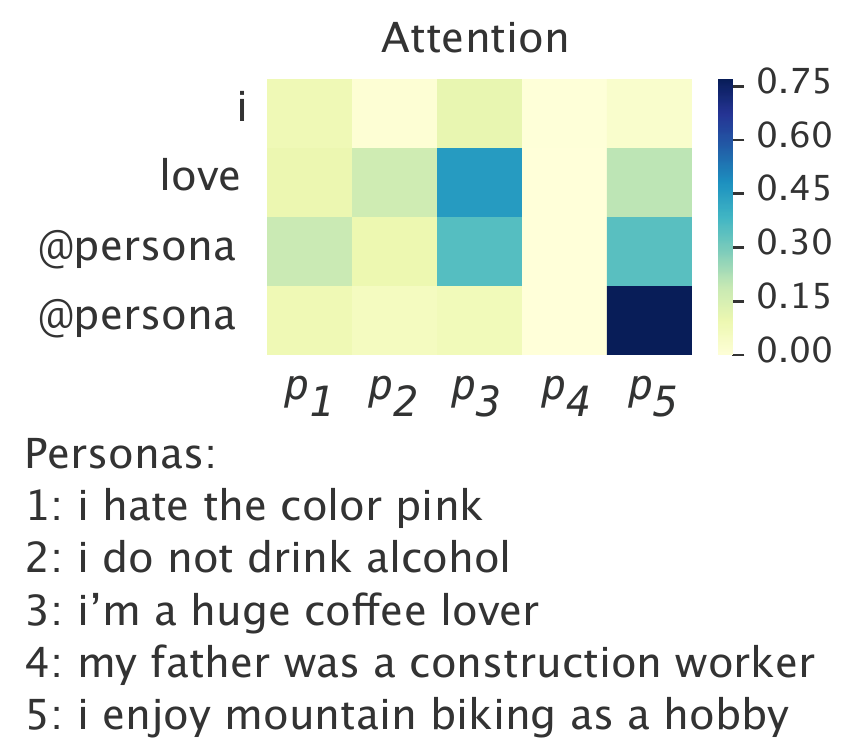}
    \end{minipage}
    \caption{Attention over memory (left) and persona traits (right). After observing ``love'', \CleverName{} attends to personas $3,5$ with related personas.}
    \label{fig:memory_attention}
\end{figure}

\begin{figure}[t!]
    \centering
    \begin{center}
    \includegraphics[width=\linewidth]{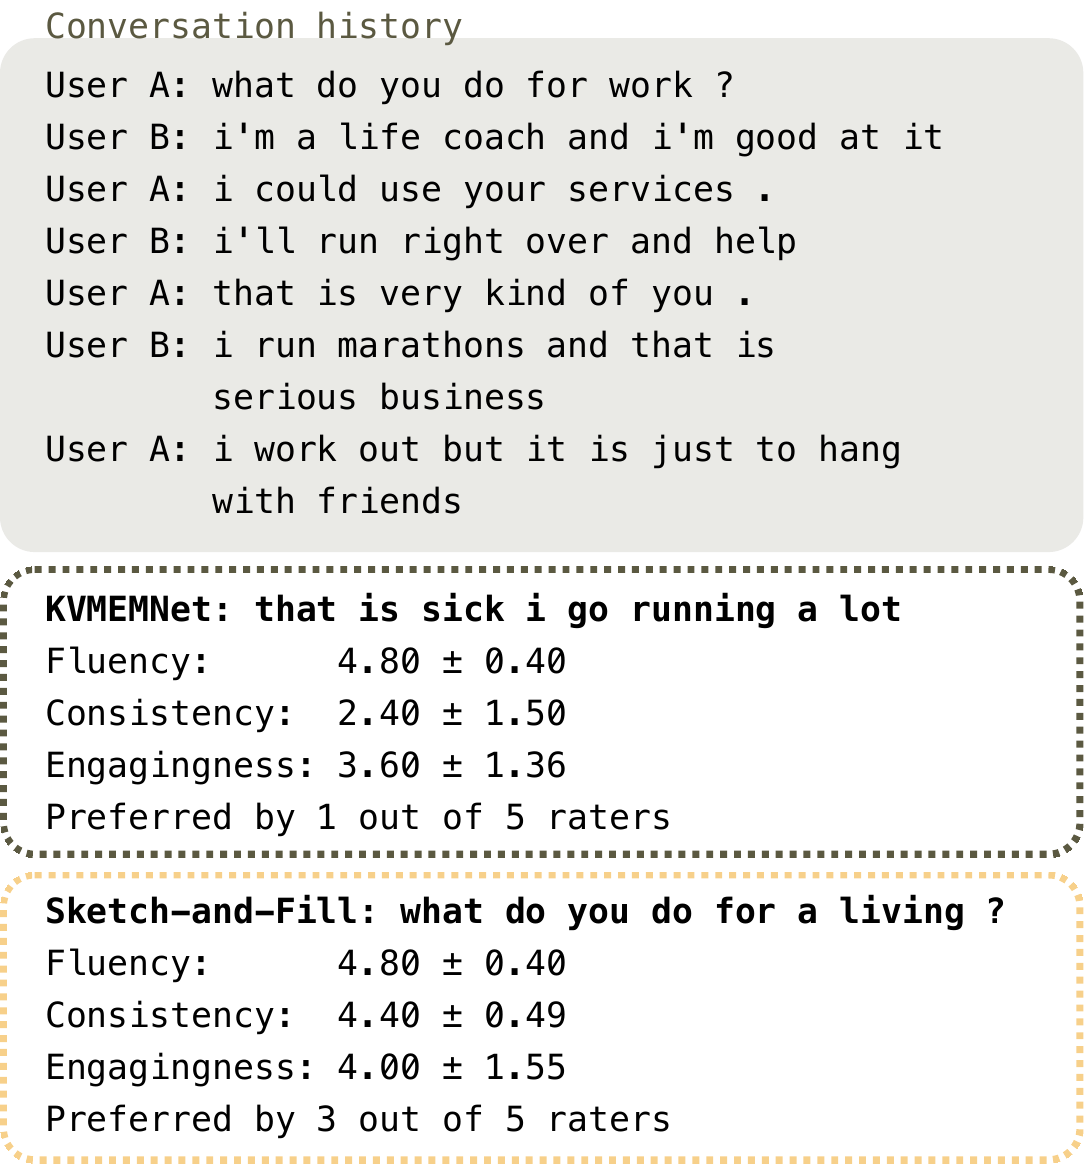}
    \end{center}
    \caption{Average ratings by 5 users for one example.}
    \label{fig:corr-pairwise}
\end{figure}

\subsection{Example Dialogues from KVMemNet}

\begin{table}
\small
\begin{tabular}{l}
Model Trait 1: I played football for a division a college \\
Model Trait 2: I enjoy poetry\\
Model Trait 3: I try various coffees as a hobby\\
Model Trait 4: I`m a huge star wars fan\\
\hline
\textbf{Human:} Hi. What do you do you for fun?.\\
\textbf{Model:} hello ! i love music i am in school to be a music teacher\\ 
\textbf{Human:} That sounds exciting! I left school a long time ago..\\ 
\textbf{Model:} i teach french\\ 
\textbf{Human:} You must be talented to teach both music and french.\\ 
\textbf{Model:} do you speak other languages ?\\
\textbf{Human:} No, just English. What about you?.\\
\textbf{Model:} i can only speak one language !\\
\textbf{Human:} Me too. Luckily we speak the same language.\\
\textbf{Model:} no do you speak another language ?\\
\textbf{Human:} No I don't speak any other languages.\\
\textbf{Model:} i do not . i do not even speak the 5 love languages\\
\textbf{Human:} I wasn't aware that there were 5 love languages.\\
\textbf{Human:} Tell me more..\\
\textbf{Model:} i speak six other languages , pick one and i will speak it\\ 
\textbf{Human:} I pick language number 3.\\
\textbf{Model:} only speak english but that is pretty cool\\
\\
\hline \hline 
\\
Model Trait 1: I enjoy coloring books \\
Model Trait 2: My husband is adopted\\
Model Trait 3: I`ve a german shepherd dog\\
Model Trait 4: I like to watch NHL hockey\\
Model Trait 5: I live is a rural farming community\\
\hline
\textbf{Human:} yo. what's up?.\\
\textbf{Model:} i am great how about you ?\\
\textbf{Human:} i am depressed.\\
\textbf{Model:} yes ! i love to dance to it . i am pretty amazing at it\\ 
\textbf{Human:} oh... that's odd. and rude...\\ 
\textbf{Human:} you want to dance to my depression?\\
\textbf{Model:} i love to dance i have moves\\
\textbf{Human:} describe your depression\\
\textbf{Model:} dance to me. i love to dance ,\\
\textbf{Model:} not to brag but i am an incredible dancer !\\
\textbf{Human:} ok. i get it. but how. alone or with others?.\\
\textbf{Model:} that is nice . no do not dance but i like to sing so...\\
\textbf{Human:} no dancing after all? you're just messing with me?\\
\textbf{Model:} yeah , dancing with my friends is my favorite .\\
\textbf{Human:} whatever man. cool .\\
\textbf{Model:} can we dance together ? i have no brothers or sisters .\\
\\
\hline \hline
\\
Model Trait 1: I have zero family that I`m close to \\
Model Trait 2: My name is George\\
Model Trait 3: My favorite food is papaya\\
Model Trait 4: I am a bee farmer\\
Model Trait 5: I married a super model from Italy\\
\hline
\textbf{Human:} hi.\\
\textbf{Model:} i am good how about you\\
\textbf{Human:} i didn't ask you that?.\\
\textbf{Model:} its pretty cool lol , tell me about you ?\\
\textbf{Human:} my favorite color is orange.\\
\textbf{Model:} oh i see that sounds cool then\\
\textbf{Human:} what about you?\\
\textbf{Model:} i hate organ lol\\
\textbf{Human:} what do u do for fun i like to go hiking.\\
\textbf{Model:} i like blue my favorite disney princess is ariel .\\
\textbf{Human:} cool, what other disney princesses do you like?.\\
\textbf{Model:} yeah disney is great . i named my 4 dogs after disney\\ characters .\\
\textbf{Model:} i like ariel becuase i have a pet fish.\\
\textbf{Human:} i love watching disney movies ! how old are you?\\
\textbf{Model:} cool my favorite color is red\\
\textbf{Human:} you're just ignoring me huh.\\
\textbf{Model:} ariel has always been my favorite\\
\end{tabular}
\caption{Multi-turn examples from KVMemNet. Model persona traits are listed before the example conversation.}
\label{tab:kvmemnet-example-3}
\end{table}

\subsection{Example Dialogues from \CleverName{}}

\begin{table}
\small
\begin{tabular}{l}
Model Trait 1: I`m a librarian \\
Model Trait 2: I really like to travel \\
Model Trait 3: I have visited Spain a times\\
Model Trait 4: I think I will retire in a few years\\
Model Trait 5: I am 60years old\\
\hline
\textbf{Human:} hi , how are you doing?. \\
\textbf{Model:} i am doing well . how about you ? \\
\textbf{Human:} i`m doing ok, i used to be an alcoholic. \\
\textbf{Model:} oh . i am sorry to hear that . \\
\textbf{Human:} tell me something about yourself. \\
\textbf{Model:} i`m a librarian . \\
\textbf{Human:} neat , what do you do as a librarian?. \\
\textbf{Model:} i work at a library . \\
\textbf{Human:} cool, what do you do for fun?. \\
\textbf{Model:} i love to read . what about you ? \\
\textbf{Human:} i like to play basketball. \\
\textbf{Model:} that sounds like fun . \\
\textbf{Human:} it is! where are you from?.\\
\textbf{Model:} i`m in the librarian .\\
\\
\hline \hline 
\\
Model Trait 1: My dream in life is to work from home \\
Model Trait 2: I dye my hair every three months \\
Model Trait 3: I went to school to be a veterinarian\\ 
but hated it\\
Model Trait 4: I have an internet addiction \\
and spend a lot of time playing roleplaying games\\
\hline
\textbf{Human:} Ciao. \\
\textbf{Model:} how are you doing tonight ? \\
\textbf{Human:} Good. Can you speak Italian?. \\
\textbf{Model:} what do you do for a living \\
\textbf{Human:} I`m a teacher. How about you?. \\
\textbf{Model:} i am a veterinarian . \\
\textbf{Human:} Do you have a dog? \\
\textbf{Model:} i do not have any pets . \\
\textbf{Human:} How do you become a vet? \\
\textbf{Model:} i am a vet . i am a vet .\\
\textbf{Human:} Do you have emergency service?\\
\textbf{Human:} Do you need to take on call?\\
\textbf{Model:} what do you like to do for fun ? \\
\textbf{Human:} Call of duty. \\
\textbf{Model:} i like to games and roleplaying time . \\
\textbf{Human:} Me too. \\
\textbf{Model:} do you have any hobbies ? \\
\textbf{Human:} Not really. \\
\textbf{Model:} i love to addiction internet .\\
\\
\hline \hline
\\
Model Trait 1: If I am not cooking in the kitchen \\
               then I am definitely on the water\\
Model Trait 2: I love cooking but I also enjoy fishing\\
Model Trait 3: Spiderman is my favorite\\
Model Trait 4: I also love comic books\\
\hline
\textbf{Human:} hi i`m [Human name]. how are you doing today ? \\
\textbf{Model:} good, has been very busy lately. \\
\textbf{Model:} what are you going to school for ? \\
\textbf{Human:} i don't go to school, i`m working. \\
\textbf{Model:} what do you do in your free time ? \\
\textbf{Human:} i play piano. \\
\textbf{Model:} i love fishing and cooking . \\
\textbf{Human:} great. \\
\textbf{Model:} what is your favorite spiderman ? \\
\textbf{Human:} i don't like spiderman. \\
\textbf{Model:} i like to enjoy . \\
\textbf{Human:} like what? \\
\textbf{Model:} spiderman is my favorite . what is your favorite ?\\
\end{tabular}
\caption{Multi-turn examples from \CleverName{}. Model persona traits are listed before the example conversation.}
\label{tab:kvmemnet-example-4}
\end{table}
